# Supplementary material for: Adaptive Private-K-Selection with Adaptive K and Application to Multi-label PATE
Source: arXiv:2203.16100 source file (2022-03-30)
Supplement: Supplementary file 1 [file appendix.tex]

\noindent\textbf{Correction.} After a revision, we spot errors in our PTR-Gaussian algorithm. We provide the correct version in Algorihm~\ref{alg: correct_ptr} where the different parts are highlighted in blue.

\begin{algorithm}[t]
	\caption{Propose-test-release (PTR) with Gaussian Mechanism}	\label{alg: correct_ptr}
	\begin{algorithmic}[1]
		\STATE{ \textbf{Input} Histogram $h(D)$, noise parameters $ \sigma_2, \sigma_3$ and the privacy parameter $\delta_t$}
		\STATE {Sort the top-$k$} Let $i_{(1)}, ..., i_{(k)}$ be the unordered indices of the sorted histogram.
		\STATE{Set the gap} $q_k = h_{i_{(k)}} -  h_{i_{(k+1)}}$
		\STATE {Propose a private lower bound of $q_k$:} $\hat{q}_k =\blue{ \max\{1,q_k\} + \cN(0, \sigma_2^2)- \sigma_2\sqrt{2\log(1/\delta_t)}}$.
		\STATE \textbf{If} $\hat{q}_k \leq 1$, \textbf{Return $\perp$}
		\STATE {Construct the indicator vector $\mathbb{I}$}: $\mathbb{I}_j =1$ if $j \in \{i_{(1)}, ..., i_{(k)}\}$ else $\mathbb{I}_j =1$.
		\STATE \textbf{If Renyi DP}, \textbf{Return} $\mathbb{I}_j + \cN(0, \sigma_3^2)$, else \textbf{Return} $\mathbb{I}$
	\end{algorithmic}
\end{algorithm}

We apply PTR-Gaussian in EXP3.  With the correct version of Algorithm~\ref{alg: correct_ptr}, we set $\sigma_2 = 25$ and  AdaTopk-Gaussian achieves $\epsilon= 5.6$.
 
In the appendix, we first state the composition and conversion rules in Sec~\ref{sec: rule}, and then provide omitted proofs in Sec~\ref{sec: proof}. The experimental details are provided in Sec~\ref{sec: exp}.

\section{Conversion and composition rules for approximated RDP}\label{sec: rule}
Recall our definition of approximate RDP.
\begin{definition}[Approximate Renyi Differential Privacy]
	We say a randomized algorithm $\cM$ is $\delta$-approximate-$(\alpha, \epsilon_\cM(\alpha))$-RDP with order $\alpha \geq 1$, if for all neighboring dataset $D$ and $D'$, there exist events $E$ (depending on $\cM(D)$ )and $E'$ (depending on $\cM(D')$) such that $\pr[E]\geq 1-\delta$ and $\pr[E']\geq 1-\delta$, and $\forall \alpha\geq 1$, we have
	$	\mathbb{D}_{\alpha}(\cM(D)|E||   \cM(D')|E')\leq  \epsilon_\cM(\alpha)$.
\end{definition}
When $\delta$ is 0, $0$-approximate-RDP is RDP.   Similar to \citep{bun2016concentrated}, the approximate-RDP satisfies the composition and post-processing property. 
\begin{lemma}[Composition rule]
	Let $\cM_1$ satisfies $\delta_1$-approximate-$(\alpha, \epsilon_{\cM_1}(\alpha))$-RDP and  $\cM_2$ satisfies $\delta_2$-approximate-$(\alpha, \epsilon_{\cM_2}(\alpha))$-RDP. Then the composition of $\cM_1$ and $\cM_2$ satisfies 
	 $(\delta_1+\delta_2)$-approximate-$(\alpha, \epsilon_{\cM_1}(\alpha)+ \epsilon_{\cM_2}(\alpha))$-RDP.
\end{lemma}
\begin{lemma}[Conversion rule]
	Let $\cM$ satisfies $\delta_1$-approximate-$(\alpha, \epsilon_{\cM}(\alpha))$-RDP. Then it also satifies $(\epsilon_\cM(\alpha)+ \frac{\log(1/\delta)}{\alpha-1}, \delta+\delta_1)$-DP.
\begin{proof}
	$\cM$ satisfies $\delta_1$-approximate-$(\alpha, \epsilon_{\cM}(\alpha))$-RDP implies that there exists an pairing event $E$ and $E'$ such that  $\mathbb{D}_\alpha (\cM(D)|E || \cM(D')|E')\leq \epsilon_{\cM}(\alpha) $ and $\pr[E]\geq 1-\delta_1, \pr[E']\geq 1-\delta_1$.
Condition on $E$ and $E'$, we apply the RDP conversion rule~\citep{mironov2017renyi}, which gives us $(\frac{\log(1/\delta)}{\alpha-1} + \epsilon_\cM(\alpha))$-DP. Then we combine the failure probability  $\delta_1$ and $\delta$, which completes the proof.
\end{proof}
\end{lemma}
\section{Omitted Proofs}\label{sec: proof}
\begin{theorem}[Restatement of Theorem~\ref{thm: rnm_k}]
	Let $\cM_g$ denote any noise-adding mechanism that satisfies $\epsilon_g(\alpha)$-RDP for a scalar function $f$ with global sensitivity $2$.  
	Assume Report-Noisy-Max adds the same magnitude of noise to each coordinate, then the algorithm obeys
	$\epsilon_\alpha(\cM(D)||\cM(D')) \leq \epsilon_g(\alpha) +\frac{\log m}{\alpha-1}$
\end{theorem}
\begin{proof}
	We use $i$ to denote any possible output of the Report-Noisy-Max $\cM(D)$. The  Report-Noisy-Max aims to select an coordinate $i$ that maximizes $C_i$ in a privacy-preserving way, where $C_i$ denotes the difference between $h_{(i)}(D)$ and $h_{(i+1)}(D)$.  Let $C'$ denote the vector of the difference when the database is $D'$. We will use the Lipschitz property: for all $j \in [m-1]$, $1+C'_j \geq j$.
			Throughout the proof, we will use $p(r_i), p(r_j)$ to denote the pdf of $r_i$ and $r_j$, where $r_i$ denote the realized noise added to the $i$-th coordinate.
	
	From the definition of Renyi DP, we have
	\begin{align}
		\mathbb{D}_\alpha(\cM(D)||\cM(D'))=\frac{1}{\alpha -1}\log \mathbb{E}_{i \sim D'}\bigg[ \frac{\pr[\cM(D)=i]^\alpha}{\pr[\cM(D')=i]^\alpha}\bigg] = \frac{1}{\alpha -1}\log \sum_{i=1}^m \frac{\pr[\cM(D)=i]^\alpha}{\pr[\cM(D')=i]^{\alpha-1}}\label{equation: rdp_def}
	\end{align}
Our goal is to upper bound $(*)= \sum_{i=1}^m \frac{\pr[\cM(D)=i]^\alpha}{\pr[\cM(D')=i]^{\alpha-1}} $.
The probability of outputting $i$ can be written explicitly as follows:
	\begin{align*}
		&\pr[\cM(D) = i] = \int_{-\infty}^\infty p(r_i) \pr[C_i + r_i > \max_{j \in [m], j \neq i} \{C_j + r_j\}] dr_i\\
		&=\int_{-\infty }^\infty p(r_i -2)  \pr[C_i + r_i -2 > \max_{j \in [m], j \neq i} \{C_j + r_j\}] dr_i\\
		&=\int_{-\infty }^\infty p(r_i) \bigg(\frac{p(r_i -2)}{p(r_i)} \bigg) \pr[C_i + r_i -2 > \max_{j \in [m], j \neq i} \{C_j + r_j\}] dr_i\\
		&= \mathbb{E}_{r_i} \bigg[ \bigg(\frac{p(r_i -2)}{p(r_i)}\bigg) \pr[C_i + r_i -2 > \max_{j \in [m], j \neq i} \{C_j + r_j\}] \bigg]  
	\end{align*}
	In the first step, the probability of $\pr[C_i + r_i > \max_{j \in [m], j \neq i} \{C_j + r_j\}]$ is over the randomness in $r_j$.
	Substituting the above expression to the definition of RDP and apply Jensen's inequality
	\begin{align*}
		&(*)= \sum_{i=1}^m \frac{ \bigg[\mathbb{E}_{r_i}  \bigg(\frac{p(r_i -2)}{p(r_i)}\bigg) \pr[C_i + p(r_i) -2 > \max_{j \in [m], j \neq i} \{C_j + r_j\}] \bigg]^\alpha}{ \bigg[  \mathbb{E}_{r_i}  \pr[C'_i + p(r_i)  > \max_{j \in [m], j \neq i} \{C'_j + r_j\}] \bigg]^{\alpha-1}}\\
		&\leq \sum_{i=1}^m\mathbb{E}_{r_i}  \bigg(\frac{p(r_i -2)}{p(r_i)}\bigg)^\alpha \bigg(\frac{ \pr[C_i + r_i -2 > \max_{j \in [m], j \neq i} \{C_j + r_j\}] }{ \pr[C'_i + r_i  > \max_{j \in [m], j \neq i} \{C'_j + r_j\}] } \bigg)^{\alpha-1} \cdot \pr[C_i + p(r_i) -2 > \max_{j \in [m], j \neq i} \{C_j + r_j\}]
	\end{align*}
We apply Jensen's inequality to bivariate function $f(x,y) = x^\alpha y^{1-\alpha}$, which is jointly convex on $\cR^2_+$ for $\alpha \in (1, +\infty)$.
	The key of the analysis relying on bounding $ (**)=\bigg(\frac{ \pr[C_i + r_i -2 > \max_{j \in [m], j \neq i} \{C_j + r_j\}] }{ \pr[C'_i + r_i  > \max_{j \in [m], j \neq i} \{C'_j + r_j\}] } \bigg)$.
	Note that $D'$ is constructed by adding or removing one user's all predictions from $D'$.
	 In the worst-case scenario, we have $C'_j = C_j +1$ for every $j \in[m], j \neq i, C_i = C'_i+1$ . Based on the Lipschitz property, we have
	\[ \pr[C'_i + p(r_i)  > \max_{j \in [m], j \neq i} \{C'_j + r_j\}] \geq  \pr[C_i + p(r_i)-2> \max_{j \in [m], j \neq i} \{C_j + r_j \}]  \]
	which implies $(**)\leq 1$.
	Therefore, we have 
	\[\epsilon_\cM(\alpha) \leq \frac{1}{\alpha-1} \log \sum_{i=1}^ m \mathbbm{E}_{r_i}  \bigg(\frac{p(r_i -2)}{p(r_i)}\bigg)^\alpha \leq \epsilon_g(\alpha) +\frac{\log(m)}{\alpha-1} . \]
\end{proof}

\begin{corollary}[Restatement of Corollary~\ref{coro_gau}]
	RNM-Gaussian (the second line in Algorithm~\ref{alg: ada-gau}) with Gaussian noise $\cN(0, \sigma_1^2)$ satisfies $(\frac{2\alpha}{\sigma_1^2}+\frac{\log m}{\alpha -1})$-RDP. 
\end{corollary}
\begin{proof}
	 For a function $f: \cD\to \cR$ with L2 sensitivity $2$,the RDP of Gaussian mechanism with Gaussian noise $\cN(0, \sigma_1^2)$ satisfies $(\alpha, \frac{2\alpha}{\sigma_1^2})$-RDP.  We complete the proof by plugging in $\epsilon_g(\alpha )= \frac{2\alpha}{\sigma_1^2}$ into Theorem~\ref{thm: rnm_k}.
\end{proof}

\begin{lemma}[Restatement of Lemma~\ref{lem: ptr}]
	Let $\hat{q}_k$ obeys $\epsilon_{gap}(\alpha)$-RDP and $\pr[\hat{q}_k \geq q_k]\leq \delta_t$ (where the probability is only over the randomness in releasing $\hat{q}_k$). If $\hat{q}_k$ passes the threshold check%\yw{It will be clearer to refer to a particular algorithm, rather than describing the algorithm informally here.}
	, the algorithm releases the set of top-$k$ indices directly satisfies $\delta_t$-approximately-$(\alpha, \epsilon_{gap}(\alpha))$-RDP. Moreover,  let  $\cM_{global}$ be any way 
	of calibrating the noise  to the global sensitivity that satisfies  $(\alpha, \epsilon_{global}(\alpha))$-RDP. If we apply $\cM_{global}$ to privately release the indicator $\mathbb{I}(D)$, then the PTR algorithm  obeys $\bigg(\alpha ,\blue{ \epsilon_{gap}(\alpha) \vee \frac{1}{\alpha-1}\log \bigg(1 -\delta_t +\delta_t e^{(\alpha-1)\epsilon_{global}(\alpha)}\bigg)}\bigg)$-RDP.
\end{lemma}
%After a careful revision, we find our statement of f Lemma~\ref{lem: ptr} in the main paper is not correct. We provide the correct version here.
The statement of Lemma~\ref{lem: ptr} in the main paper has a typo and we provided the correct version of it above (the changes are highlighted in blue).

\begin{proof}
	We start with the proof for $\delta_t$-approximately-$(\alpha, \epsilon(\alpha))$-RDP. 
	Denote $\cM_{1}$ be the mechanism that releases the set of top-$k$ indices directly (without adding noise) if $\hat{q}_k$ passes the threshold check ($\hat{q}_k>1$).%  Let $S_1$  be the range of $\cM_1(D)$, which is either $\perp$ or an indicator $\mathbb{I}(D) \in \{0,1\}^m$. Let $E_1$ be the measurable set of $\hat{q}_k$ that represents the event $\hat{q}\leq q_k$, i.e., the high-probability lower bound of $q_k$ is valid. Check that $\P[E_1]\geq 1-\delta$ for any input dataset. 
	
	Then let us discuss the two cases of the neighboring pairs $D,D'$.
	\begin{enumerate}[label=(\alph*)]
		\item For neighboring datasets $D,D'$ where the Top-$k$ indices are the same, the possible outputs are therefore $\{\perp, \mathrm{Top-k}(D)\}$ for both $\cM_1(D),\cM_1(D')$. Notice that $|q_k(D)-q_k(D')| \leq 1$, thus in this case 
		$$
		\mathbb{D}_\alpha(\cM_1(D) \| \cM_1(D'))= D_\alpha(\mathbf{1}(\hat{q}_k(D)>1) \| \mathbf{1}(\hat{q}_k(D')>1) ) \leq \mathbb{D}_\alpha(\hat{q}_k(D)\|\hat{q}_k(D') ) \leq \epsilon_{gap}(\alpha),	$$
		where the inequality follows from the information-processing inequality of the Renyi Divergence.
		%algorithm's binary output is a post-processing of the mechanism that releases $\hat{q}_k$.  
		Thus it trivially satisfies $\delta$-approximated-$(\alpha,\epsilon_{gap}(\alpha))$-RDP when we set $E$ to be the full set, i.e., $\Pr[E]=1 \geq 1-\delta$.
		\item For $D,D'$ where the Top-$k$ indices are different, then it implies that $q_k(D)\leq 1$ and $q_k(D')\leq 1$. In this case, we can construct $E$ to be the event where $\hat{q}_k\leq q_k$, i.e., the high-probability lower bound of $q_k$ is valid. Check that $\P[E]\geq 1-\delta$ for any input dataset.  Conditioning on $E$,  $\hat{q}_k \leq q_k \leq 1$ for both $D,D'$, which implies that $\Pr[\cM_1(D) = \perp | E] = \Pr[\cM_1(D') = \perp | E] = 1$. Thus, trivially $\mathbb{D}_{\alpha}(\cM(D) | E(D) \| \cM(D') | E(D') ) =0$ for all $\alpha$. For this reason, it  satisfies $\delta$-approximated-$(\alpha,\epsilon(\alpha))$-RDP for any function $\epsilon(\alpha)\geq 0$, which we instantiate it to be $\epsilon_{gap}(\alpha)$.
%		Consider $D,D'$ such that $q_k(D) = 2$ and  $q_k(D')=1$. The Top-$k$ indices are the same, so the output space of both datasets are $\{\perp, \textrm{Top-k-index}(D) \}$.  Conditioning on $E_1$, i.e., $\hat{q}_k\leq q_k$.  For $D$,  
%		$$\Pr_{\cM(D)}[\hat{q}_k \geq 1  | \hat{q}_k \leq  q_k] = \Pr_{\cM(D)}[\hat{q}_k \geq 1  | \hat{q}_k \leq  2]  > 0$$
%		However for $D'$, 
%		$$
%		\Pr_{\cM(D')}[\hat{q}_k \geq 1  | \hat{q}_k \leq  q_k]  = \Pr_{\cM(D)}[\hat{q}_k \geq 1  | \hat{q}_k \leq  1]  = 0.
%		$$
%		Thus $D_{\alpha}[ \cM(D)|E_1(D) \| \cM(D') | E_1(D') ]  = +\infty$ for all $\alpha > 0$.
	\end{enumerate}
	
%	First of all, releasing $\hat{q}_k$ obeys $(\alpha, \epsilon_{gap}(\alpha)$)-RDP.
%	Conditional on $E_1$, we have $\forall o \in S_1$, 
% \[\pr[\cM_1(D)=o|E_1]  = \pr[\cM_1(D')=o|E_1]\]
% This is because when $\hat{q}_k \leq 1$, $\cM_1(D) = \cM_1(D') = \perp$, else $\cM_1(D) = \cM_1(D') =\{0, 1\}^{m}$. Therefore, $\cM_1$ satisfies $\delta_t$-approximately-$(\alpha, 0)$-RDP. By the composition rule, we have releasing $\hat{q}_k$ and $\cM(D)$ obeys $\delta_t$-approximately-$(\alpha, \epsilon_{gap}(\alpha))$-RDP.
% 
 We now consider the alternative version where we get a (pure) RDP guarantee when we apply $\cM_{global}$ to privately release the indicator $\mathbb{I}(D)$ if $\hat{q}_k$ passes the threshold check.
% To achieve a pure RDP, we consider a slight modification of Algorithm~\ref{alg: correct_ptr} by setting $\hat{q}_k = \max\{1,q_k\} + \cN(0, \sigma_2^2)- \sigma_2\sqrt{2\log(1/\delta)}$.  
We denote this process as $\cM_2$ and  denote $S_2$ as the range of $\cM_{2}(D)$. 
 
 We will again discuss the two cases.  In Case (a), the Top-K indices are the same for $D,D'$, thus the Renyi-divergence of the two outputs $\cM_{global}$ is $0$ even if it is being executed.  Thus the Renyi-divergence is bounded by $\epsilon_{gap}(\alpha)$ as discussed before.

 In Case (b), the Top-K indices are different for $D,D'$,  $q_k(D)\leq 1$ and $q_k(D')\leq 1$, thus $\hat{q}_k$ has the same distribution between $D,D'$. Define event $E$ to be $\hat{q}_k\leq 1$.  We know that under both $D,D'$, $\Pr[E]= 1-\delta$. 
 
  Follow the definition of RDP, we have
 \[\mathbb{D}_\alpha(\cM_{2}(D)|| \cM_2(D')) = \frac{1}{\alpha-1} \log \mathbb{E}_{o \sim \cM(D')} \bigg[\frac{\pr[\cM_2(D)=o]^\alpha}{\pr[\cM_2(D')=o]^\alpha}\bigg]\]
 
\begin{align*}
&\E_{o \sim \cM(D')} \bigg[\frac{\pr[\cM_2(D)=o]^\alpha}{\pr[\cM_2(D')=o]^\alpha}\bigg] \\
=&  \frac{\pr[\cM_2(D)=\perp]^\alpha}{\pr[\cM_2(D')=\perp]^{\alpha-1}} + \sum_{o}  \pr[\cM_2(D')\neq\perp]\pr[
\cM_{global}=o] \left(\frac{\pr[\cM_2(D)\neq\perp]\pr[
	\cM_{global}(D')=o]}{\pr[\cM_2(D')\neq\perp]\pr[
	\cM_{global}(D')=o]}\right)^\alpha\\
=&1-\delta + \delta \E_{o\sim \cM_{global}(D')}\left[ \left(\frac{\pr[
	\cM_{global}(D)=o]}{\pr[
	\cM_{global}(D')=o]}\right)^\alpha\right]\\
=&1-\delta + \delta e^{(\alpha-1)\epsilon_{global}(\alpha)}.
\end{align*}

The RDP is therefore bounded by $$\max\left\{ \epsilon_{gap}(\alpha) , \frac{1}{\alpha-1}\log(1-\delta + \delta e^{(\alpha-1)\epsilon_{global}(\alpha)})\right\}.$$

\end{proof}
\begin{lemma}
	PTR-Laplace outputs $k$ elements with probability at least $1-\beta$,  if we have $h_{(k)} - h_{(k+1)}\geq 1+\log(1/\delta_t)/\epsilon + \log(1/\beta)/\epsilon$.
\end{lemma}
We correct the typo  in Remark~2: the gap requirement is $1 + 2 \log(1/\delta)/\epsilon$ instead of $1 + 1 \log(1/\delta)/\epsilon$.
\begin{proof}
With $q_k \geq  1+\log(1/\delta_t)/\epsilon + \log(1/\beta)/\epsilon$, we have 
\[\hat{q}_k \geq  1 + \log(1/\delta_t)/\epsilon + \log(1/\beta)/\epsilon + \mathrm{Lap}(1/\epsilon) - \log(1/\delta_t)/\epsilon =  \log(1/\beta)/\epsilon +1 + \mathrm{Lap}(1/\epsilon) \]
PTR-Laplace outputs $k$ elements only when $\hat{q}_k>1$.
Therefore, the failure probability is bounded by $\pr[\mathrm{Lap}(1/\epsilon)> \log(1/\beta)] =\beta$.
\end{proof}

   \begin{theorem}[Restatement of Theorem~\label{thm: t_composition}]
	Assume Algorithm~\ref{alg: ada-lap} satisfies $\delta_t$-approximately-$(\alpha,  \alpha \epsilon^2)$-RDP. Then Algorithm~\ref{alg: fix_k} obeys $\tilde{T}\delta_t$-approximately-$(\alpha, \tilde{T}\alpha\epsilon^2)$-RDP.
	%Let $\tilde{C}_j = h_{(j)} - h_{(j+1)}+\lambda|j-k|$ denotes the utility of the $j$-th candidate. In the unrestricted setting, we add independently generated Laplace noise to each candidate and release the index of the largest noisy count as well as its noisy count. The algorithm satisfies $\epsilon$-DP.
\end{theorem}
\begin{proof}
	We apply the composition rule of approximated-RDP and that completes the proof.
\end{proof}
\section{Experimental details}\label{sec: exp}
In this section, we provide more details for the experiments.
 
 In EXP3, BrightKite~\citep{cho2011friendship} contains over $100000$ users and $1280000$ candidates.  Foursquare~\citep{yang2014modeling} contains $2293$ users with over $100000$ c andidates. 
 In EXP3, we implement PATE with $\sigma=80$.  For PATE-$\tau$, we follow the implementation in \citet{zhu2020private} with $\tau =10$.
%\begin{comment}
\section{Generalized to float count}
\subsection{Smooth Sensitivity}
Let $f(D)\in \{0,1\}^n$ denote the non-private output of the algorithm $f$ at dataset $D$,  which is a $0, 1$ vector and only the $k$ selected indexes $i_{(1)}, ..., i_{(k)}$ are set to $1$. We first recall the definition of the local sensitivity.
\begin{definition}[Local Sensitivity]
	For $f: \cD^n \to \{0,1\}^n$ and $D\in \cD^n$, the local sensitivity of $f$ at $D$ (with respect to the $\ell_1$ metric) is
	\[LS_f(D) =\max_{D': d(D,D')=1} ||f(D) - f(D')||_1 \]
\end{definition}
$d(D, D')=1$ says that two datasets differ one user's data. Algorithm~\ref{alg: ls} calculates the local sensitivity in time $O(k)$. The idea behind the algorithm is that: by changing one user's data, the count gap between two adjacent element can decrease by at most $2$. Thus, if the gap between $h_{i_{k}}$ and $h_{i_{k+1}}$ is greater or equal to $2$, the local sensitivity is $0$. For other cases, we define two pointers $\ell$ and $j$ that start at $k+1$. The goal is to maximize the integral such that $h_{i_{\ell}} -h_{i_{j}}\leq 1$ and the local sensitivity will be $\min\{k+1 -\ell, j - (k+1)\}$.

Note that the global sensitivity is $GS_f = \max_D LS_f(D)$, which is $k$ in our case.
Moreover, the sensitivity of $f$ at distance $d$ is \[A^{(d)}(D) = \max_{D' \in \cD:d(D, D')=d}LS_f(D')\]. 

% first say how to compute it when d = 0

For any $D$, the local sensitivity at distance $d$ is maximized when the entries $h_{i_{k+1}}, ..., h_{i_{2k}}$ are still remained as an non-decreasing sequence while the hamming distance among the adjacent entries is minimized. Algorithm~\ref{alg: ad} returns $A^{(d)}(D)$ at distance $d$. The intuition is, when the gap between the $k$-th and the $k+1$-th is greater than $2d$, the local sensitivity will be always $0$. In other cases, the worst-case would be $h_{i_{k}} = h_{i_{k+1}}$ and the gap between the adjacent entries is minimized (i.e., $\min_{h} \sum_{j=1}^{2k-1} |h_{i_{j}} - h_{i_{j+1}}|$). 

Now smooth sensitivity can be expressed in terms of $A^{(d)}(D)$.
\begin{definition}
	The $\beta$-smooth sensitivity $S^*_{f, \beta}(D)$ is defined as:
	\[S^*_{f, \epsilon}(D) = \max_{d=0, ..., m} e^{-d\beta}\bigg(\max_{D': d(D,D')=d}LS_f(D')\bigg)=\max_{d = 0, ..., m}e^{-d\beta}A^{(d)}(D)\]
\end{definition}

\begin{algorithm}[t]
	\caption{Local Sensitivity $LS_f(D)$}
	\label{alg: ls}
	\begin{algorithmic}[1]
		\STATE $\ell =  j = k+1$
		\STATE \textbf{While} $h_{i_{(\ell)}} = h_{i_{(\ell-1)}}$ and $\ell\geq 2$, $\ell =\ell-1$\\
		\STATE $\ell \gets \ell -1$ if $h_{i_{(\ell-1)}} =h_{i_{(\ell)}}+1$\\
		\STATE \textbf{While} $h_{i_{(j)}} = h_{i_{(j+1)}}$ and $j\leq m-1$, $j=j+1$\\
		\STATE $j \gets j+1$ if $h_{i_{(j+1)}} =h_{i_{(j)}}-1$\\
		\STATE \textbf{Return} $\min\{k+1 -\ell, j - (k+1)\}$
	\end{algorithmic}
\end{algorithm}

\begin{algorithm}[t]
	\caption{Calculate $A^{(d)}(D)$}
	\label{alg: ad}
	\begin{algorithmic}[1]
		\STATE{ \textbf{Input} $D, d, k$}
		\STATE \textbf{If} $h_{i_{k}} - h_{i_{k+1}} \geq 2d$ \textbf{Return 0}
		\STATE $h_{i_{(k)}}=h_{i_{(k+1)}} = \lfloor (h_{i_{(k)}} + h_{i_{(k+1)}})/2 \rfloor $
		\STATE \textbf{For} $\ell =k-1 \text{  to  } 1$
		\STATE $h_{i_{(\ell)}} = \max(h_{i_{(\ell+1)}}, h_{i_{(\ell)}} -d )$ 
		\STATE \textbf{For} $j =k+1 \text{  to  } 2k$
		\STATE $h_{i_{(j)}} = \min(h_{i_{(j-1)}}, h_{i_{(j)}} +d )$ 
		\STATE Construct $D'$ using $h$.
		\STATE \textbf{Return}($LS_f(D')$) using Algorithm~\ref{alg: ls}
	\end{algorithmic}
\end{algorithm}
\yq{}{Add one example here}

Moreover, we can upper bound the smooth sensitivity using global sensitivity, speeding up the computation when $d$ is large.
\begin{lemma}
	For a given value $d_0(n)$, let 
	\[\hat{S}_{f,\epsilon}(D) =\max (GS_f \cdot e^{-\epsilon d_0}, \max_{d = 0,..., d_0 -1}e^{-\epsilon d}\cdot A^{(d)}(D)) \]
\end{lemma}
$GS_f$ is $k$ in our case.
\subsection{Calibrate noise with respect to smooth sensitivity}
\begin{lemma}
	Let $h$ be an $(\alpha, \beta)$-admissible noise probability density function, and let $Z$ be a fresh random variable sampled according to $h$. For a function $f: D^n \to \mathbbm{R}^d$, let $S: D^n \to \mathbbm{R}$ be a $\beta$-smooth upper bound on the local sensitivity of $f$. Then algorithm $\cA(x) = f(x) + \frac{S(x)}{\alpha}\cdot Z$ is $(\epsilon, \delta)$-differential private.
\end{lemma}
\begin{example}\label{exp: gaussian}
	Let $Z$ samples from the $n$-dimensional Gaussian distribution $\cN(0, I_m)$. Consider a dataset $D$ where $A^{(d_0)}(D)=0$ for a fixed $d_0\geq 0$. Take $\alpha =\frac{\epsilon}{5\sqrt{2\ln(2/\delta)}}$ and $\beta =\frac{\epsilon}{4(2k+\ln(2/\delta))}$. The algorithm $\cA(x) = f(d) + \frac{ke^{-\beta d_0}}{\alpha} \cdot Z$ is $(\epsilon, \delta)$-DP. 
\end{example}
Compared to the Gaussian mechanism using the global sensitivity only, this example amplifies the standard deviation of noise addition by $O(e^{-\beta d_0})$.

\begin{comment}
\section{Report Noisy Max}

%Let $C_{j}(D)$ denote the difference between $h_{i_{j}}$ and $h_{i_{(j+1)}}$. We want to output the index of the largest $C_{j}(D)$ and the corresponding noisy count. 
In the Report Noisy Max algorithm, we add independently generated Laplace noise $Lap(1/\epsilon)$ to each $C_{j}$ and return the index of the largest noisy count and the corresponding noisy count.
\begin{theorem}[Report Noisy Max with Laplace noise]
	The Report Noisy Max algorithm is $(\epsilon, 0)$-differentially private.
\end{theorem}
\begin{proof}
	The first part of the proof on reporting the noisy index is copied from the original proof and the second part on reporting the noisy max count is an extenstion of the first part.
	
	Fix $D = D' \cap x_i$. Let $C_{j}$, respectively $C_{j}'$ denote the shorthand of  $C_{j}(D)$ and $C_{j}(D')$. The following two properties hold.
	\begin{enumerate}
		\item Monotonicity of Counts. For all $j \in [m], c_j \geq c_j'$.
		\item Lipschitz Property. For all $j \in [m], 1 + C_j' \geq C_j$.
	\end{enumerate}
	When each user can at most modify $m$ bins by $1$, the above properties still holds.
	Fix any $i \in [m]$. Let $r^{-i}$ denote the Laplace noise $Lap(1/\epsilon)^{m-1}$ used for $C$ and $C'$ except the $i$th coordinate. We will bound from above and below the ratio of the probabilities that $i$ is selected with $D$ or with $D'$.
	We use the notation $\pr[i |\cdot]$ to mean the probability that the ouput of the Report Noisy Max algorithm is $i$, conditioned on $\cdot$.
	We first argue that $\pr[i| D', r_{-i}]\leq e^{\epsilon}\pr[i|D, r_{-i}]$.
	For $\forall j \in [m] \neq i$, let $r^* = \min_{r_i} C_i + r_i > C_j + r_j$. 
	Note that, having fixed $r_{-i}$ , $i$ will be the output when the dataset is $D$ if and only if $i\geq r^*$.  Moreover, we have 
	\[ 1+ C_i' + r^* \geq C_i + r^*  > C_j + r_j \geq C_j' + r_j\]
	Thus, if $r_i \geq r^* +1$, then $i$ will be the output when the database is $D'$.
	Therefore, we have
	\[\pr[i| D', r_{-i}] = \pr[r_i \geq r^* +1] \geq e^{-\epsilon} \pr[r_i \geq r^*] = e^{-\epsilon} \pr[i|D, r_{-i}]  (*)\]
	We now consider $\pr[i| D, r_{-i}]\leq e^{\epsilon}\pr[i|D', r_{-i}]$.
	Define 
	\[r^* = \min_{r_i} C_i' +r_i > C_j' + r_j \forall j\neq i \leq m\]
	We have 
	\begin{align*}
		C_i' + r^*  &>C_j' + r_j\\
		C_i' + r^* + 1 &> C_j' + r_j + 1\\
		C_i' + r^* + 1 &> C_j' + r_j + 1\geq C_j + r_j\\
		C_i + (r^* +1) \geq C_i' + r^* + 1 &> C_j' + r_j + 1\geq C_j + r_j\\
	\end{align*}
	Thus, if $r_i \geq r^* +1$, $i$ will be the output on database $D$. We therefore have, 
	\[\pr[i |D, r_{-i}] = \pr[r_i \geq r^* +1] \geq e^{-\epsilon} \pr[r_i \geq r^*] = e^{-\epsilon} \pr[i| D', r_{-i}]\]
	
	We next argue that the release of the maximum noisy count incurs no further loss of privacy.  We use $pdf(r_i)$ to denote the pdf of $r_i$. 
	Condition on the $r_{-i}$ and the ouput index is $i$, let $y$ be the noisy max count, i.e. $y = C_i + r_i$.
	Then we have 
	\[\frac{\pr[y| D, r_{-i}]}{\pr[y| D', r_{-i}]} = \frac{p(y-C_i)}{p(y - C'_i)} = \frac{p(r_i)}{p(r_i+C_i-C'_i)}\leq \frac{p(r_i)}{p(r_i +1)} (**)\]
	Our next step is to show that privately releasing $i$ implies $ \frac{p(y-C_i)}{p(y - C'_i)}\leq e^{\epsilon}, \forall y$.
	From $(*)$, we know that $\pr[i|D', r_{-i}]\geq \pr[r_i \geq r^* +1]\geq e^{-\epsilon} \pr[i|D, r_{-i}]$, where we can rewrite the probability in the following integration form:
	\[\pr[r_i \geq r^* +1] = \int_{r^*+1}^\infty p(r_i)dr_i\]
	Therefore, we have
	\[= \int_{r^*+1}^\infty p(r_i)dr_i \geq e^{-\epsilon} \int_{r^*}^\infty p(r_i) dr_i\]
	By changing the integration variable, we have
	\[= \int_{r^*}^\infty p(r_i+1)dr_i \geq e^{-\epsilon} \int_{r^*}^\infty p(r_i) dr_i\]
	We now differentiate the left and the right part, which gives us
	\[ p(r_i+1) \geq e^{-\epsilon}  p(r_i)\]
	Plug in the equation above into $(**)$, which completes the proof.
\end{proof}
When we replace Laplace noise with Gaussian noise, the RDP bound of releasing the noisy max index is provided in the following lemma.
\begin{theorem}
	
	In the user-vote scheme (each user can modify at most $m$ coordinates), we denote $\cM_g$ be noise-adding mechanism that satisfies $\epsilon_g(\alpha)$-RDP with global sensitivity 1.  In other settings where neighboring dataset can differ by $\triangle$ in at most one coordinate, we denote 
	$\cM_g$ be noise-adding mechanism that satisfies $\epsilon_g(\alpha)$-RDP with global sensitivity $\triangle$.
	Assume Report Noisy Max adds the same magnititude of noise to each coordinate, then Report Noisy Max obeys
	\[\epsilon_\alpha(\cM(D)||\cM(D')) \leq \epsilon_g(\alpha) +\frac{\log m}{\alpha-1}\]
\end{theorem}

In the utility guarantee of Report Noisy Max, the question that we want to answer is ``with Gaussian noise drawn from $\cN(0, \sigma^2)$, if the gap between the largest $C_i$ and the second-largest $C_i$ is greater than $d_c$, what is the failure probabiliy that the output index is not $i$.

\section{Utility Analysis}
This section first provides the utility bound of our method and then compares our utility with two state-of-the-art private k selection methods. Our analysis is based on a specific setting where all methods can amplify their privacy analysis.

In the comparison, the privacy budget is fixed to $(\epsilon, \delta)$. We compare the minimum gap between $h_{i,k}$ and $h_{i,k+1}$, such that with probability at least $1-\beta$, the algorithm outputs the correct $k$ indexs. 
Denote the calibrated Gaussian noise be $\cN(0,\sigma_1^2)$ and gap between $h_{k}$ and $h_{k+1}$ is greater than $\tilde{T}$. The goal is to find a $\tilde{T}$ such that the probability of outputting the correct top $k$ index is greater than $1-\beta$. Denote $X_1, j \in{1, ...,k}$ be the event that the $j$-th largest index is not included in the algorithm. Therefore,  we can bound the failure probability \[\pr[X_1\cup X_2, ... \cup X_k ]\leq \beta\]. Given that $X_j$ is independent to each other, it is equivalent to construct a $\tilde{T}$ such that $\pr[X_j ]\leq \beta/k$ and then apply the union bound.
\begin{align}
	\pr[X_i \leq \beta/k] &= \pr\bigg[h_{i_{(j)}}+ \cN(0, \sigma_1^2)\geq  h_{i_{(k+1)}}+\cN(0, \sigma_1^2)\bigg]\\
	&= \pr\bigg[h_{i_{(j)}} - h_{i_{(k+1)}} \geq  \cN(0, \sigma_1^2) -\cN(0, \sigma_1^2) \bigg]\\
	&= \pr\bigg[h_{i_{(j)}} - h_{i_{(k+1)}} \geq  \cN(0, \sigma_2^2) \bigg]\\
	&\leq \pr \bigg[ h_{i_{(k)}} - h_{i_{(k+1)}} \geq \cN(0, \sigma_2^2)\bigg]\\
	&\leq \pr \bigg[ \cN(0, \sigma_2^2) \geq \tilde{T}\bigg]
\end{align}
where $\sigma_2^2 =2\sigma_1^2$. 
\yq{}{The correct first step shall be $\pr[h_{i_{(j)}}+ \cN(0, \sigma_1^2)\geq  \max_{t>0} h_{i_{(k+t)}}+\cN(0, \sigma_1^2)$  }
Applying the tail bound og Gaussian distribution, we have 
\[\pr \bigg[ \cN(0, \sigma_2^2) \geq \tilde{T}\bigg]\leq e^{\frac{-\tilde{T}^2}{2\sigma_2^2}}\leq \frac{\beta}{k}\]
which implies \[\frac{\tilde{T}}{\sigma_2}\geq \sqrt{\frac{\log(k/ \beta)}{2}}\]
Example~\ref{exp: gaussian} suggests that it  is sufficient to take $\sigma_2 = \sqrt{2}\sigma_1= \sqrt{2}\frac{ke^{-\beta_0 d_0}}{\alpha} \cdot Z$, where the the dilation parameter $\beta_0 =\frac{\epsilon}{4(d+\ln(2/\delta))}$ , the sliding parameter $\alpha=\frac{\epsilon}{5\sqrt{\log(2/\delta)}}$ and $d_0$ describes how many entries of $D$ are modified when the local sensitivity approaches the  global sensitivity.  Note that the  gap is greater than $\tilde{T}$ which implies $d_0\geq \tilde{T}+k$. \red{Moreover, as the output of our algorithm is the top $k$ index, we can set $d = k$}. Substituting $\alpha, \beta$ into $\sigma_2$, which gives us the following result
\begin{align}
	&\frac{\tilde{T}}{\sigma_2} \geq \sqrt{\frac{\log(k/\beta)}{2}}\equiv 	\frac{\tilde{T}}{\sigma_1} \geq \sqrt{\log(k/\beta)}\\
	&\equiv \frac{\alpha \tilde{T}e^{\beta_0  d_0}}{k} \geq \sqrt{\log(k/\beta)}\\
	&\equiv \frac{\epsilon \tilde{T} e^{\frac{\epsilon (\tilde{T}+k)}{k+\log(2/\delta)}}}{k\sqrt{\log(2/\delta)}}\geq \sqrt{\log(k/\beta)}\\
	&\equiv  \tilde{T} e^{\frac{\epsilon (\tilde{T}+k)}{k+\log(2/\delta)}}\geq \frac{k \sqrt{\log(k/\beta)\log(2/\delta)}}{\epsilon}
\end{align}
To make the inequality states, it suffices to consider $\tilde{T} = O(\frac{\sqrt{\log(2/\delta)\log(k/\beta)}}{\epsilon})$.

The baseline methods is provided below.
\textbf{TS~\citep{carvalho2020differentially}}:  TS is a stability-based method. 
\begin{theorem}[Theorem 4.1~\citep{carvalho2020differentially}]
	\textbf{TS} outputs $k$ elements with probability at least $1-\beta$, if for any given $i$ such that $k\leq i\leq \bar{k}$ we have $h_i - h_{i+1}\geq 1+ (\log(\bar{k}/\delta)+\log(1/\beta)/(\epsilon/4))$, where $(\epsilon,\delta)$ is the privacy parameter.
\end{theorem}
end{comment}
